# Supplementary material for: Theory for the Acoustic Raman Modes of Proteins
Source: arXiv:1608.01279 source file (2016-08-03)
Supplement: Supplementary file 1 [file TheoryAcousticModesProtein_DeWolfGordon_SuppInfo.pdf]

# Supporting Information for "An Elastic Network Model for the Acoustic Raman Modes of Proteins"

Timothy DeWolf and Reuven Gordon
*Department of Electrical and Computer Engineering,*
*University of Victoria, British Columbia, Canada**
(Dated: June 7, 2016)

### Protein Names

Some of the proteins used here have alternate names: bovine pancreatic trypsin inhibitor is also known as aprotinin; ovotransferrin is also known as conalbumin; and, cyclooxygenase is also known as prostaglandin-endoperoxide synthase.

### The Anisotropic Network Model

The anisotropic network model (ANM) calculates the Hessian matrix [2]

$$H = \begin{pmatrix} \mathcal{H}_{11} & \mathcal{H}_{12} & \cdots & \mathcal{H}_{1N} \\ \mathcal{H}_{21} & & & \mathcal{H}_{2N} \\ \vdots & & \ddots & \vdots \\ \mathcal{H}_{N1} & \mathcal{H}_{N2} & \cdots & \mathcal{H}_{NN} \end{pmatrix}. \tag{1}$$

The $i, j = 1...N$ index the $N$ atoms in the system. The result of computing the Hessian second derivatives for this network of springs is given by the matrix product [2, 3]

$$\mathcal{H}_{ij} = -\frac{k}{s_{ij}^2} \begin{pmatrix} x_j - x_i \\ y_j - y_i \\ z_j - z_i \end{pmatrix} \begin{pmatrix} x_j - x_i & y_j - y_i & z_j - z_i \end{pmatrix} \tag{2}$$

($i \neq j$). For $\mathcal{H}_{ii}$ and $\mathcal{H}_{jj}$, this same $\mathcal{H}_{ij}$ is subtracted from any existing diagonal entries as the loop over all pairs inside radius $r_c$ is executed [3]. $s_{ij}$ measures the Cartesian distance between atoms and $i$ and $j$; $k$ is the spring constant. The $\{x_i, y_i, z_i\}$ are atomic equilibrium coordinates (from the PDB file) of the atoms in the protein.

In the paper (see also Table 1 in the paper), we calculate a spring constant $k$ for each protein. We indicated that this is achieved by "matching the atomic mean-square fluctuations predicated by ANM...with the crystallographic isotropic temperature factors." Details of this calculation follow. The atomic mean-square fluctuations (MSF) $\langle(\Delta R_i)^2\rangle$ are found using

$$\langle(\Delta R_i)^2\rangle = \frac{3B_i}{8\pi^2}, \tag{3}$$

where the $B_i$ are the crystallographic temperature factors or B-factors (stored in the PDB file along with the crystal coordinate measurements) for each atom $i$ [4].

Protein thermal fluctuations have also been studied using the Gaussian network model (GNM), another single-parameter (the spring constant) potential model [5]. It builds upon established theories of elastic networks, also termed phantom rubber networks [6]. Extending these ideas to ANM, ProDy provides a utility function that calculates an estimate of $\langle(\Delta R_i)^2\rangle$. (It uses a result from statistical mechanics to estimate a variance for each mode; this is multiplied by the Cartesian norm of each atomic displacement in the unit eigenvector. A summation over all modes is performed.)

One must correctly select the stiffness of the ANM spring constant $k$ such that the ANM-computed $\langle(\Delta R_i)^2\rangle$ best match those found using the B-factors. We integrate the area under the experimental (crystal) and theoretical (ANM) MSF curves ($\langle(\Delta R_i)^2\rangle$ vs $i$), and use interpolation to determine $k$.

### The Ellipsoid Polarizability Calculation

The two mode-displaced coordinate sets are generated with $\vec{r}_{i,\pm} = \vec{r}_0 \pm \beta\vec{Q}_i$. We use $\beta = 0.0001$ Å for all our calculations; as noted, $\vec{Q}_i$ is a unit vector in $\mathbb{R}^{3N}$. One can check if $\beta$ is small enough by computing Raman spectra over a wide range of $\beta$. Values of $\beta$ where the whole spectrum scales together are small enough; at some point $\beta$ becomes large enough that scanning over $\beta$ yields nonlinear behavior where different modes scale independently with $\beta$. (As $\beta$ increases, some interatomic distances become unphysical, e.g. far outside of the allowed C-C bond length.)

The ellipsoid that "best fits" a collection of point masses, such as our mode-displaced protein coordinates $\vec{r}_{i,\pm}$, is found using the following technique [7]. One recognizes that the moment of inertia tensor for a collection of point masses may be written as [8]

$$I_{\alpha\beta} = \sum m_i(r_i^2\delta_{\alpha\beta} - r_{i,\alpha}r_{i,\beta}) \tag{4}$$

with $r_i = (x_i^2 + y_i^2 + z_i^2)^{1/2}$. The inertia tensor for uniform mass $M$ ellipsoid with semi-principle axes $a$, $b$ and $c$ is

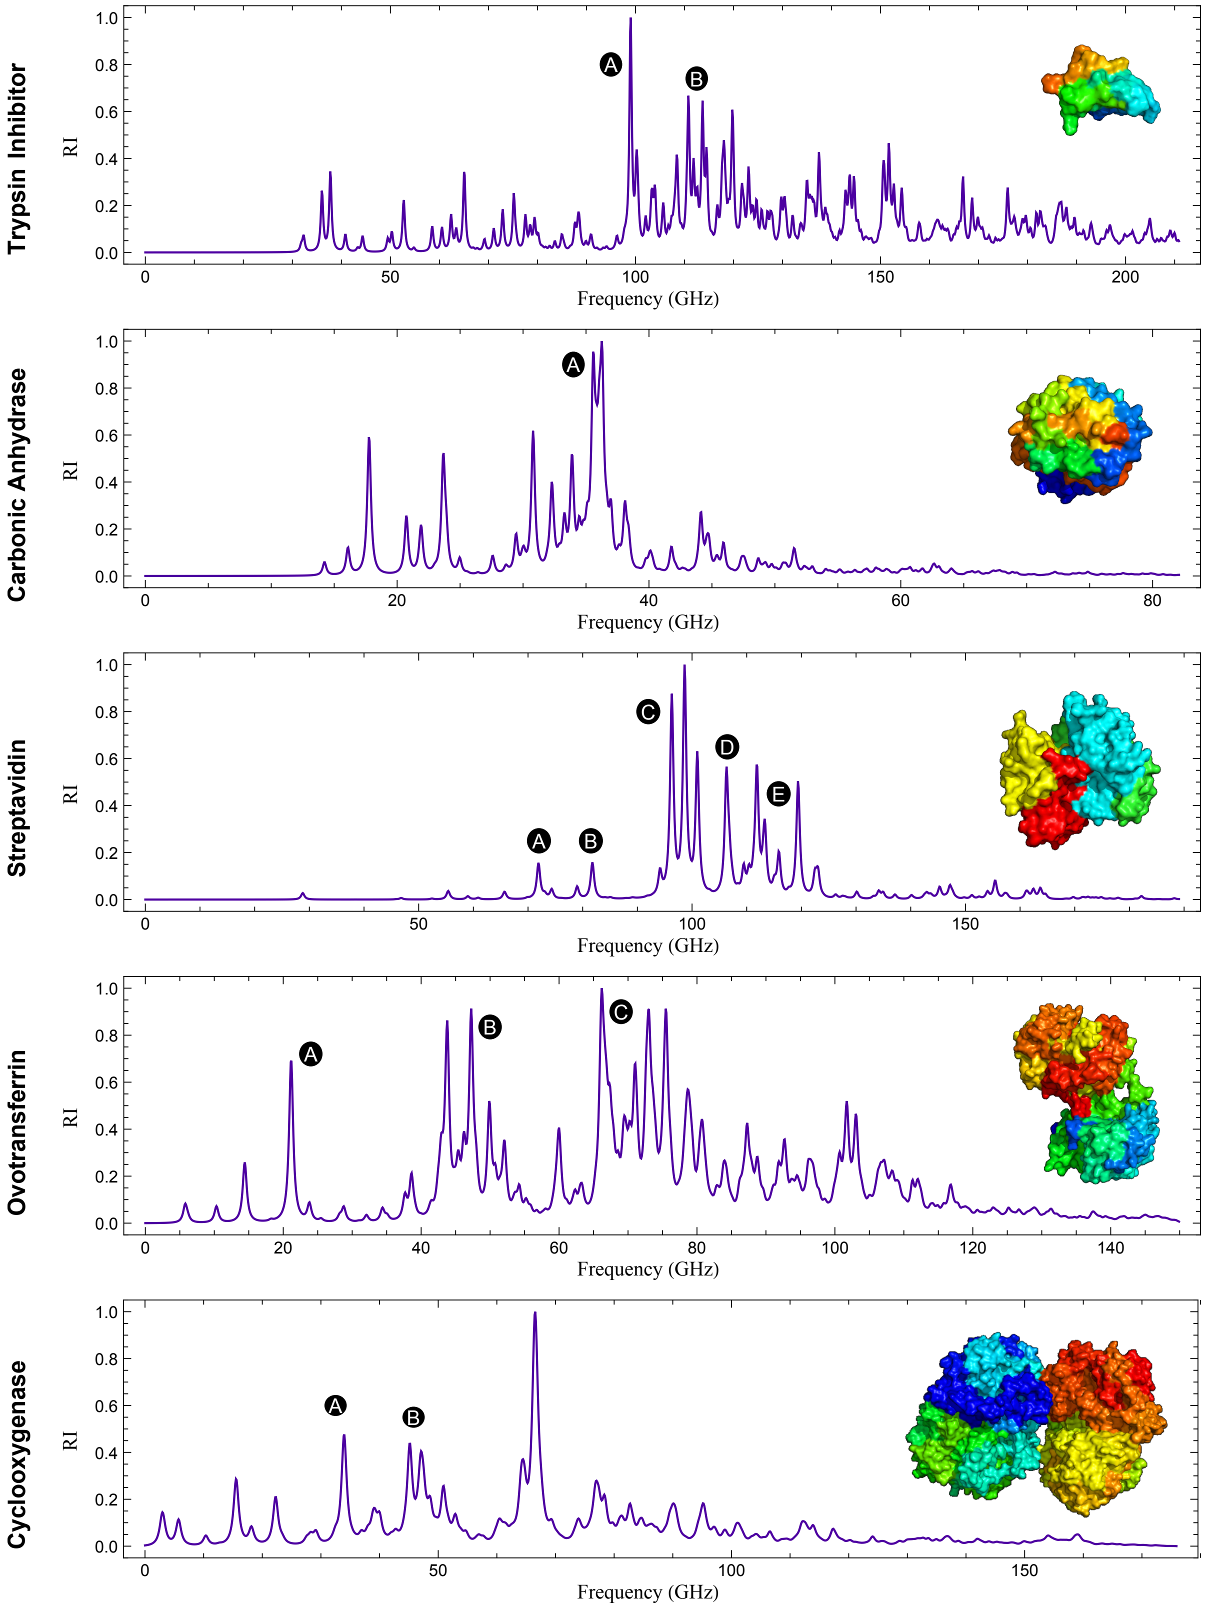


FIG. 1: Larger spectral window of the theoretical Raman intensity (RI) calculation. Compare with Fig. 2 in the paper; the same major peak labels are preserved. Inset protein images generated using PyMOL [1].

equated with Eq. 4, and the following relation results

$$\frac{M}{5}\begin{pmatrix}(b^2+c^2) & 0 & 0\\ 0 & (a^2+c^2) & 0\\ 0 & 0 & (a^2+b^2)\end{pmatrix}$$
$$= \frac{M}{5}(a^2+b^2+c^2) - \sum_i m_i \vec{r}_i \otimes \vec{r}_i \rightarrow \quad (5)$$

$$\sum_i m_i \vec{r}_i \otimes \vec{r}_i = \frac{M}{5}\begin{pmatrix}a^2 & 0 & 0\\ 0 & b^2 & 0\\ 0 & 0 & c^2\end{pmatrix}. \quad (6)$$

This result means that the eigenvalues and eigenvectors of the $3\times3$ tensor $\Omega_{\alpha\beta} = \sum_i m_i r_{i,\alpha} r_{i,\beta}$ are related to the semi-principle axis lengths $a$, $b$, $c$ and axis unit vectors $\hat{u}_a$, $\hat{u}_b$, $\hat{u}_c$.

The polarizability tensor $\alpha$ of a uniform electric permittivity dielectric ellipsoid is given by [9, 10]

$$\alpha = \frac{4\pi\, abc}{3} \sum_{j=x,y,z} \frac{\epsilon_0\epsilon_e(\epsilon_i-\epsilon_e)}{\epsilon_e + N_j(\epsilon_i-\epsilon_e)} \hat{u}_j\hat{u}_j. \quad (7)$$

The factor of $4\pi\, abc/3$ out front is the ellipsoid volume. The internal and external relative permittivities are $\epsilon_i = n^2 = 1.6^2$ and $\epsilon_e = 1.33^2$. The $\hat{u}_j$ are Cartesian unit vectors, aligned with the ellipsoid semi-principle axes. The $N_j$ are depolarization factors, which account for the ellipticity of the ellipse. The depolarization factors can be expressed concisely as an single analytic integral, but to simplify numerical evaluation they can be expressed as [9, 10]

$$N_x = \frac{abc}{(a^2-b^2)\sqrt{a^2-c^2}}(F(\phi,m) - E(\phi,m)) \quad (8)$$
$$N_y = 1 - N_x - N_z \quad (9)$$
$$N_z = \frac{b}{b^2-c^2}\left(b - \frac{ac}{\sqrt{a^2-c^2}}E(\phi,m)\right) \quad (10)$$
$$m = \frac{a^2-b^2}{a^2-c^2}, \quad \phi = \arccos\frac{c}{a}. \quad (11)$$

Many numerical software packages (we use SciPy [11]) provide implementations of the incomplete elliptic integrals of the first and second kind, denoted here by F and E:

$$F(\phi,m) = \int_0^\phi \frac{\mathrm{d}\psi}{\sqrt{1-m\sin^2\psi}} \quad (12)$$
$$E(\phi,m) = \int_0^\phi \sqrt{1-m\sin^2\psi}\,\mathrm{d}\psi. \quad (13)$$

These expressions require $a > b > c$, so the semi-principle axes obtained from diagonalization of the protein inertia tensor must be sorted. Rotational degrees of freedom do not appear in the mode vectors $\vec{Q}_k$, but there is a possibility that the semi-principle axes of the best-fit ellipsoid could rotate between the two mode extremes. The analytic polarizability does not account for this possibility, so we compute the rotation matrix [8]

$$R = \begin{pmatrix}\hat{u}_{a,+}\cdot\hat{u}_{a,-} & \hat{u}_{a,+}\cdot\hat{u}_{b,-} & \hat{u}_{a,+}\cdot\hat{u}_{c,-}\\ \hat{u}_{b,+}\cdot\hat{u}_{a,-} & \hat{u}_{b,+}\cdot\hat{u}_{b,-} & \hat{u}_{b,+}\cdot\hat{u}_{c,-}\\ \hat{u}_{c,+}\cdot\hat{u}_{a,-} & \hat{u}_{c,+}\cdot\hat{u}_{b,-} & \hat{u}_{c,+}\cdot\hat{u}_{c,-}\end{pmatrix} \quad (14)$$

and rotate $\alpha^+$ as a general rank 2 tensor, $\alpha_{+,\mathrm{rot}} = R^{\mathrm{T}}\alpha_+ R$. The important quantity $\alpha'_i = (\partial\alpha_i/\partial Q_i)_0$ [12] is then approximated by $\alpha' \approx \alpha_{i,+,\mathrm{rot}} - \alpha_{i,-}$.

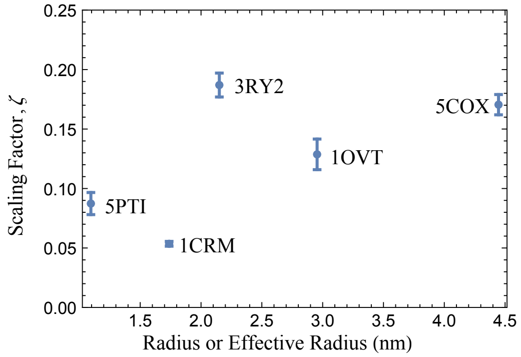


FIG. 2: The scaling factor $\zeta$ for the five proteins; the scaling factor relates the EAR mode frequencies $\tilde{\omega}_i$ to ANM frequencies $\omega_i$. Protein radius is estimated using the radius of gyration [3]; likely, both radius and protein structure contribute to $\zeta$. ANM (vacuum) frequencies are consistently lower than the water-solvated protein frequencies measured via EAR.

## The Theoretical Spectra

The theoretical spectra are constructed by summing a set of Lorentzian functions [13], one for each eigenmode $i$ with frequency $\omega_i$:

$$\mathrm{RI}(\omega) = \sum_i \frac{\Gamma}{2\pi}\frac{1}{(\omega-\omega_i)^2 + (1/2\,\Gamma)^2}; \quad (15)$$

$\Gamma$ is the linewidth (FWHM). The values of $\Gamma$ used are 0.57 GHz, 0.34 GHz, 0.74 GHz, 0.7 GHz and 1.04 GHz for the five proteins 5PTI, 1CRM, 3RY2, 1OVT and 5COX respectively.

As discussed, the EAR mode frequencies $\tilde{\omega}_i$ and ANM frequencies $\omega_i$ are approximately linearly proportional: $\tilde{\omega}_i = \zeta\omega_i$ at the chosen cut-off value $r_c$; the required values of the scaling parameter $\zeta$ are given in Fig. 2.

In Fig. 1 we show a wider spectral window for the low-frequency acoustic modes for the five proteins studied in the paper.

The protein refractive index $n_i = 1.6$ is an approximation, but our $n_i$ agrees, within $\pm0.3$, with published values [14]. To assess the robustness of the theory with respect to minor changes in refractive index, Fig. 3 shows Raman spectra calculated using our theory for three values of refractive index. The theoretical spectra diverge

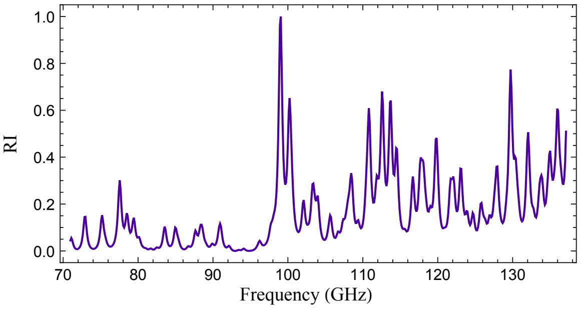


(a) $n_i = 1.5$.

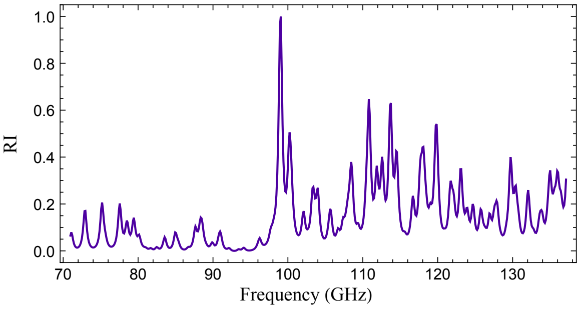


(b) $n_i = 1.6$.

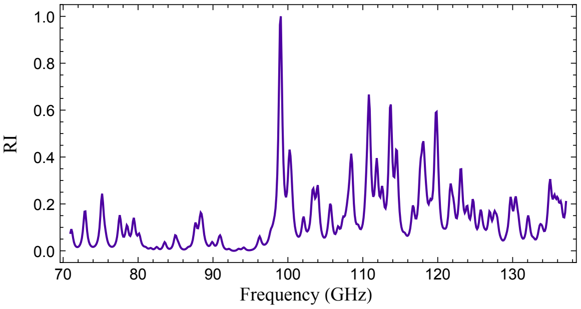


(c) $n_i = 1.7$.

FIG. 3: Calculated Raman intensity spectra for different values of protein refractive index ($n_i$) for the protein 5PTI. The spectra are quite stable under changes in protein refractive index (except when the protein index approaches the index of the surrounding water).

substantially as $n_i$ approaches the index of water, but otherwise remain quite stable even up to high refractive index values ($n_i \gg 1.6$).

Fig. 4 shows a sample of the eigenmodes for 5PTI. As seen, the lower frequency modes tend to feature collective motions involving all of the atoms in the protein to nearly equal extents, while the higher frequency modes exhibit localized displacements primarily involving only a small number of atoms. Note that the elastic network (single-parameter) models like ANM reliably reproduce the dynamics of only the slower modes, e.g. modes with $f \lessapprox 450$ GHz [15].

* Electronic address: rgordon@uvic.ca

[1] Schrödinger, LLC, *The PyMOL Molecular Graphics System, Version 1.3, Schrödinger, LLC.* (2010), [Online; accessed 2016-04-05], URL http://www.pymol.org/.

[2] P. Doruker, A. R. Atilgan, and I. Bahar, Proteins: Structure, Function, and Bioinformatics **40**, 512 (2000), ISSN 1097-0134, URL http://dx.doi.org/10.1002/1097-0134(20000815)40:3<512::AID-PROT180>3.0.CO;2-M.

[3] A. Bakan, L. M. Meireles, and I. Bahar, Bioinformatics **27**, 1575 (2011), URL http://bioinformatics.oxfordjournals.org/content/27/11/1575.abstract.

[4] A. Atilgan, S. Durell, R. Jernigan, M. Demirel, O. Keskin, and I. Bahar, Biophysical Journal **80**, 505 (2001), ISSN 0006-3495, URL http://www.sciencedirect.com/science/article/pii/S000634950176033X.

[5] I. Bahar, A. R. Atilgan, and B. Erman, Folding and Design **2**, 173 (1997), ISSN 1359-0278, URL http://www.sciencedirect.com/science/article/pii/S1359027897000242.

[6] D. S. Pearson, Macromolecules **10**, 696 (1977), URL http://dx.doi.org/10.1021/ma60057a040.

[7] H. Jang-Condell and L. Hernquist, The Astrophysical Journal **548**, 68 (2001), URL http://stacks.iop.org/0004-637X/548/i=1/a=68.

[8] L. Hand and J. Finch, *Analytical Mechanics* (Cambridge University Press, 1998).

[9] A. Sihvola, *Electromagnetic Mixing Formulas and Applications*, Electromagnetics and Radar Series (Institution of Electrical Engineers, 1999).

[10] E. C. Stoner, The London, Edinburgh, and Dublin Philosophical Magazine and Journal of Science **36**, 803 (1945), URL http://dx.doi.org/10.1080/14786444508521510.

[11] E. Jones, T. Oliphant, P. Peterson, et al., *SciPy: Open source scientific tools for Python* (2001–), [Online; accessed 2016-04-05], URL http://www.scipy.org/.

[12] L. Woodward, in *Raman Spectroscopy: Theory and Practice*, edited by H. A. Szymanski (Plenum Press, 1967).

[13] Eric W. Weisstein, *"Lorentzian Function." From MathWorld–A Wolfram Web Resource*, [Online; accessed 2016-04-05], URL http://mathworld.wolfram.com/LorentzianFunction.html.

[14] T. L. McMeekin, M. Wilensky, and M. L. Groves, Biochemical and Biophysical Research Communications **7**, 151 (1962), ISSN 0006-291X, URL http://www.sciencedirect.com/science/article/

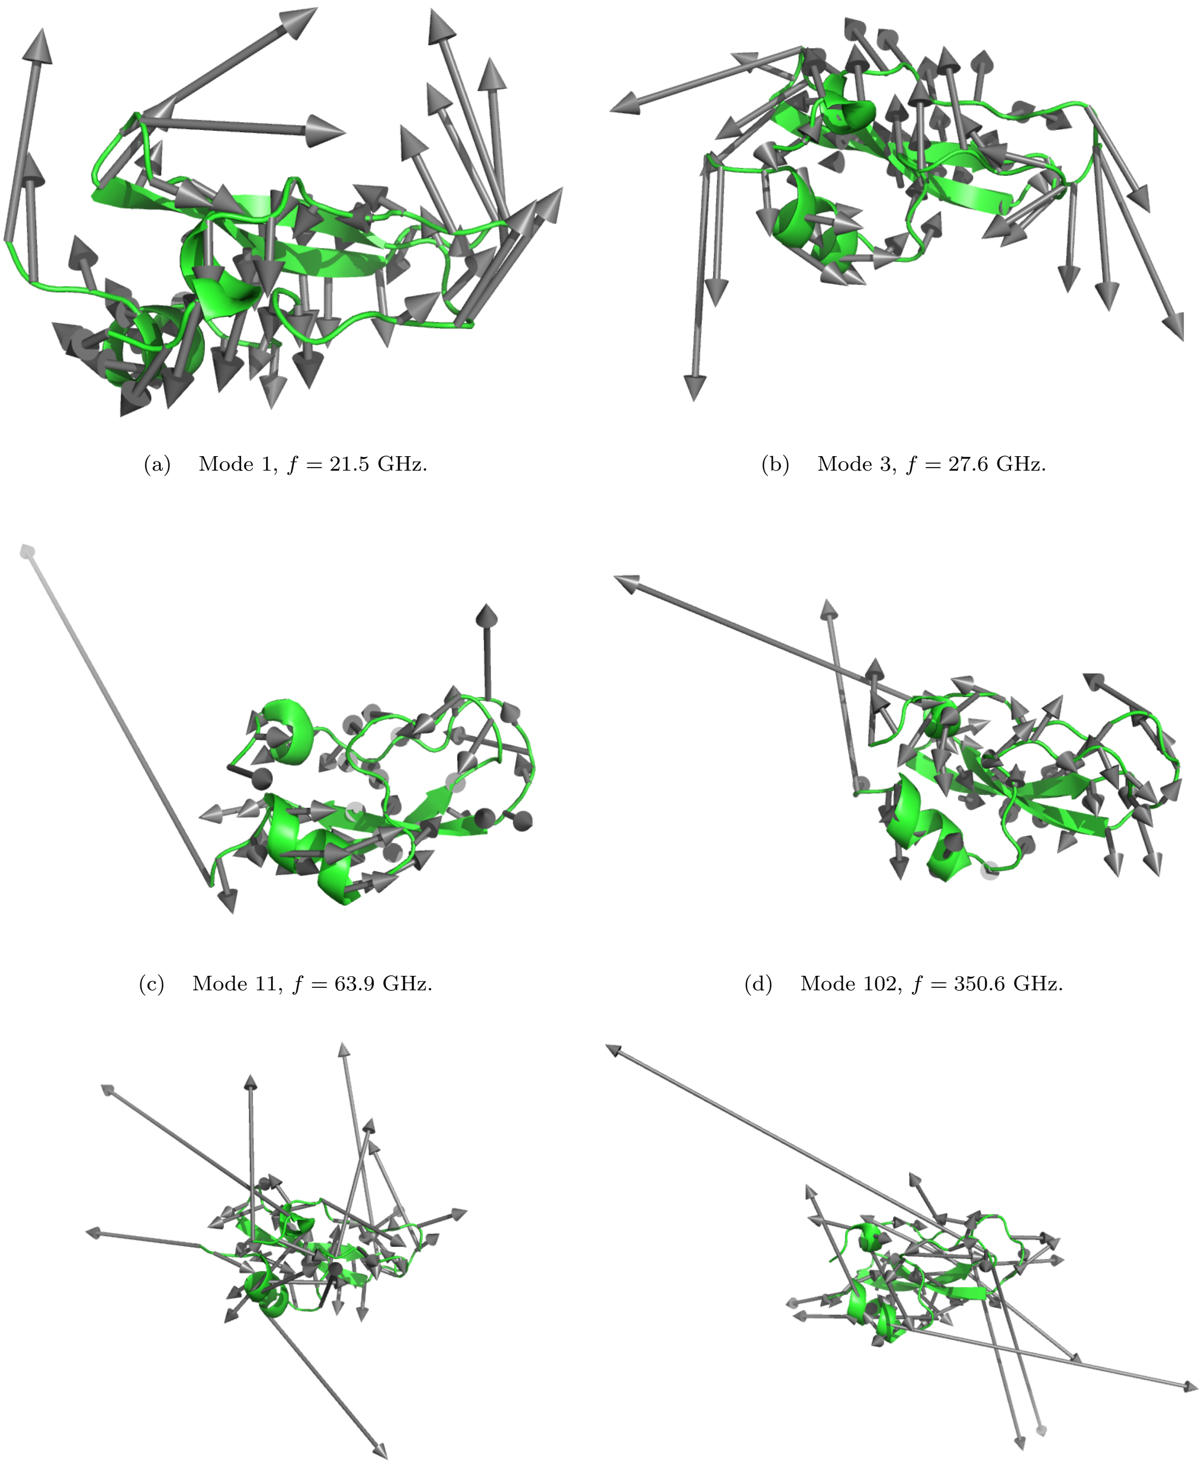

(a) Mode 1, $f = 21.5$ GHz.

(b) Mode 3, $f = 27.6$ GHz.

(c) Mode 11, $f = 63.9$ GHz.

(d) Mode 102, $f = 350.6$ GHz.

(e) Mode 202, $f = 586.6$ GHz.

(f) Mode 1002, $f = 1405.8$ GHz.

FIG. 4: Some eigenvectors of the all-atom, $r_c = 7.9$ Å, ANM Hessian matrix for the small protein 5PTI. The observed trend is that the lower frequency eigenvectors are highly collective, whereas the higher frequency modes feature localized displacements. The length of the displacement vector components (the gray arrows in $\mathbb{R}^3$) are highly exaggerated; small amplitude components have been omitted. The protein (green) is shown in a cartoon representation that highlights residues having an $\alpha$-helix or $\beta$-sheet character.

pii/0006291X62901651.
[15] M. M. Tirion, Phys. Rev. Lett. **77**, 1905 (1996), URL http://link.aps.org/doi/10.1103/PhysRevLett.77.1905.
